# Supplementary material for: Semiconductor to metal transition in bilayer phosphorene under normal compressive strain
Source: arXiv:1412.2116 source file (2014-12-30)
Supplement: Supplementary file 1 [file supp.pdf]

# Supplementary Information for Nanotechnology:
# Semiconductor to metal transition in bilayer phosphorene under normal compressive strain

Aaditya Manjanath[†,‡,¶], Atanu Samanta[†,¶], Tribhuwan Pandey[†,¶], and Abhishek K. Singh[*†]

[†]Materials Research Centre, Indian Institute of Science, Bangalore-560012
[‡]Centre for Nano Science and Engineering, Indian Institute of Science, Bangalore-560012
[¶]These authors contributed equally to this work

## 1 Supplementary Tables

Table S1: Calculated structural parameters of bilayer phosphorene using PBE+vdW

| $a$ (Å) | $b$ (Å) | $d$ (Å) | $\delta_1$ (Å) | $\delta_2$ (Å) | $\alpha_1/\alpha_1'$ (°) | $\alpha_2/\alpha_2'$ (°) |
|---|---|---|---|---|---|---|
| 4.45 | 3.35 | 3.23 | 2.26 | 2.23 | 102.62/102.63 | 97.1/97.0 |

Table S2: In-plane stiffness, effective masses, deformation potential and room temperature carrier mobilities as a function of normal compressive strain. The values of NC strain, $C_{sx}$ and $C_{sy}$ are repeated for the convenience.

| Carrier type | Normal compression (%) | $C_{sx}$ (Nm$^{-1}$) | $C_{sy}$ (Nm$^{-1}$) | $m_x^*/m_0$ | $m_y^*/m_0$ | $E_{1x}$ (eV) | $E_{1y}$ (eV) | $\mu_x$ ($10^3$ cm$^2$V$^{-1}$s$^{-1}$) | $\mu_y$ ($10^3$ cm$^2$V$^{-1}$s$^{-1}$) |
|---|---|---|---|---|---|---|---|---|---|
| hole | 0.00 | 52.79 | 212.488 | 0.1028 | 2.039 | 2.720 | 1.462 | 3.237 | 2.275 |
| | 0.83 | 52.26 | 208.363 | 0.1202 | 1.900 | 2.642 | 1.500 | 2.783 | 2.178 |
| | 1.66 | 52.35 | 207.424 | 0.1209 | 1.764 | 2.706 | 1.650 | 2.732 | 1.996 |
| | 2.49 | 52.37 | 204.318 | 0.1216 | 1.653 | 2.790 | 1.850 | 2.631 | 1.720 |
| | 3.32 | 51.88 | 205.167 | 0.1226 | 1.562 | 2.496 | 1.988 | 3.314 | 1.622 |
| | 4.15 | 51.45 | 203.480 | 0.1242 | 1.497 | 2.460 | 2.296 | 3.388 | 1.276 |
| | 4.98 | 51.42 | 200.763 | 0.1268 | 1.474 | 2.372 | 2.824 | 3.559 | 0.843 |
| electron | 0.00 | 52.79 | 212.488 | 0.1108 | 1.297 | 1.606 | 4.81 | 10.400 | 0.399 |
| | 0.83 | 52.26 | 208.363 | 0.1319 | 1.306 | 1.640 | 4.992 | 7.581 | 0.329 |
| | 1.66 | 52.35 | 207.424 | 0.1334 | 1.316 | 1.680 | 4.974 | 7.082 | 0.325 |
| | 2.49 | 52.37 | 204.318 | 0.1352 | 1.327 | 1.604 | 5.032 | 7.579 | 0.307 |
| | 3.32 | 51.88 | 205.167 | 0.1381 | 1.339 | 1.880 | 5.116 | 5.275 | 0.290 |
| | 4.15 | 51.45 | 203.480 | 0.1433 | 1.354 | 1.932 | 5.140 | 4.664 | 0.276 |
| | 4.98 | 51.42 | 200.763 | 0.1535 | 1.369 | 2.024 | 5.054 | 3.809 | 0.267 |

*abhishek@mrc.iisc.ernet.in

## 2 Supplementary Figures

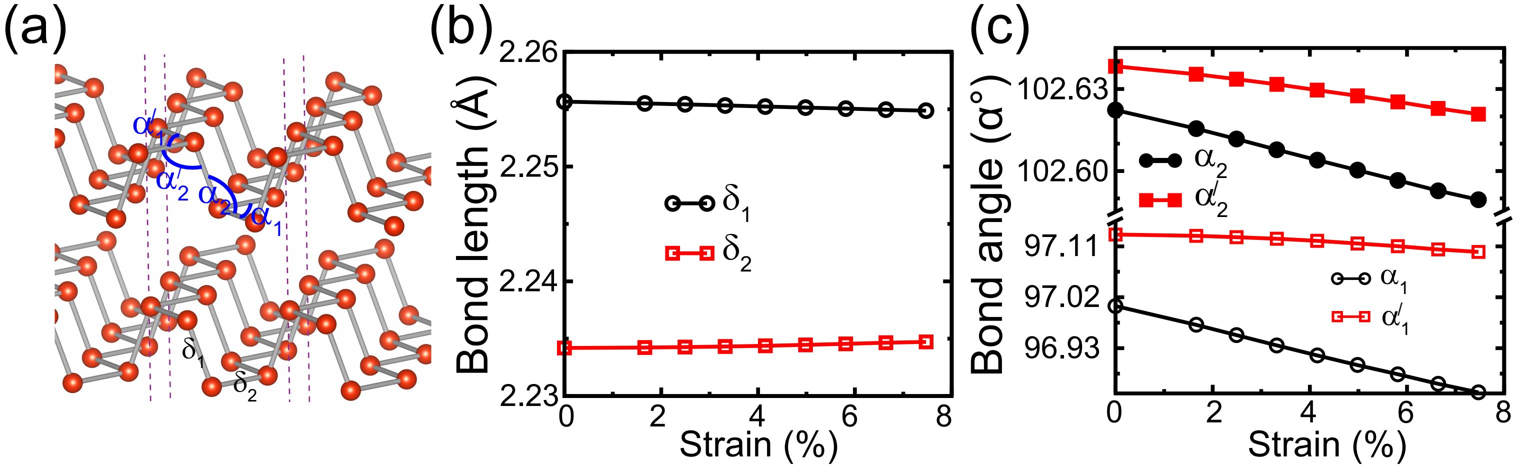


Figure S1: The crystal structure of bilayer phosphorene marked with structural parameters: bond angles $\alpha_1$, $\alpha_1'$, $\alpha_2$, $\alpha_2'$ and bond distances $\delta_1$, $\delta_2$. (b) Evolutions of the bond lengths and (c) bond angles (as marked in the figure (a)) with respect to the applied NC strains.

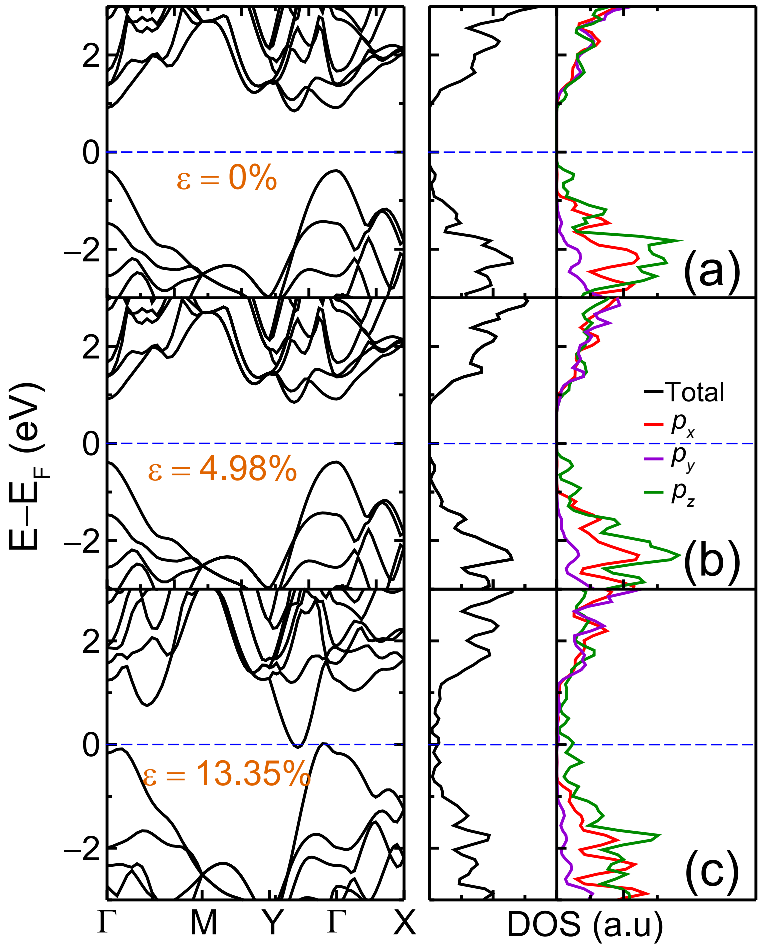


Figure S2: Band structures of bilayer phosphorene calculated with HSE06 functional at (a) $0\%$, (b) $4.98\%$, and (c) $13.35\%$ normal compressions with corresponding total (colored black) and LDOS (colored lines). Fermi level is set to 0 (blue-dashed line).

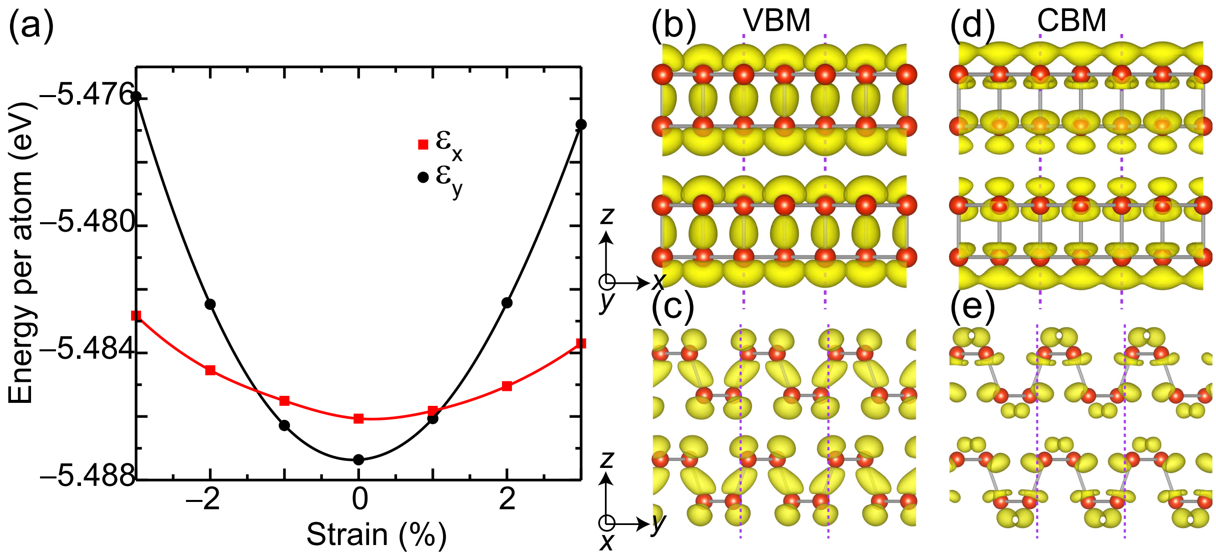


Figure S3: (a) Energy per atom of bilayer phosphorene at $3.32\%$ compression as a function of in-plane strain along $x$- and $y$-directions. Band-decomposed charge density plots of VBM and CBM for bilayer phosphorene are shown in (b)-(e), where (b) and (c) corresponds to VBM plots along $x$- and $y$-directions, and (d) and (e) corresponds to CBM plots along $x$- and $y$-directions, respectively.

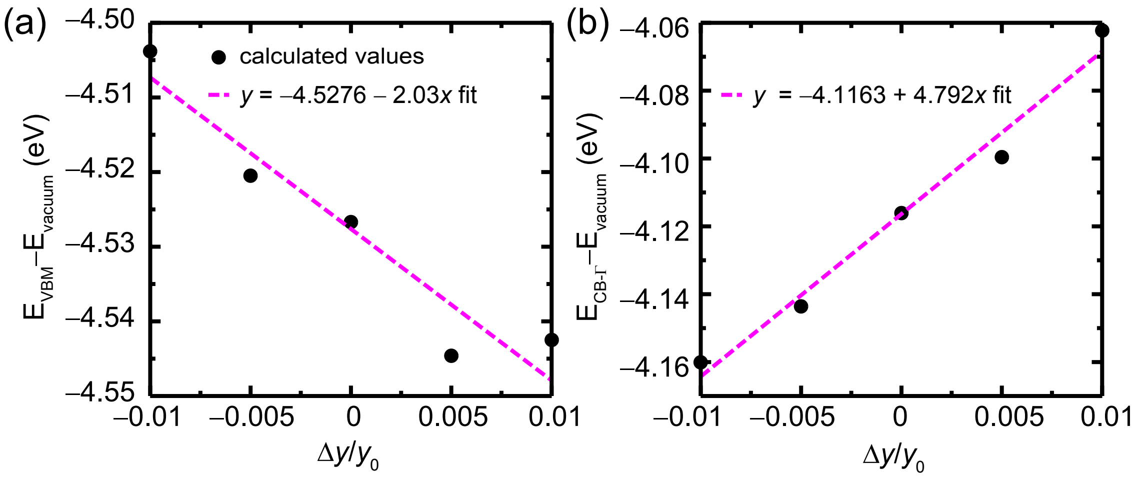


Figure S4: Band energy of the (a) VBM and (b) CB at Γ of bilayer phosphorene, with respect to the vacuum energy as a function of lattice dilation. Band energies were calculated with the PBE functional. Pink dotted lines are the linear fits. The slope of these plots gives the deformation potential $E_{1\alpha}$.

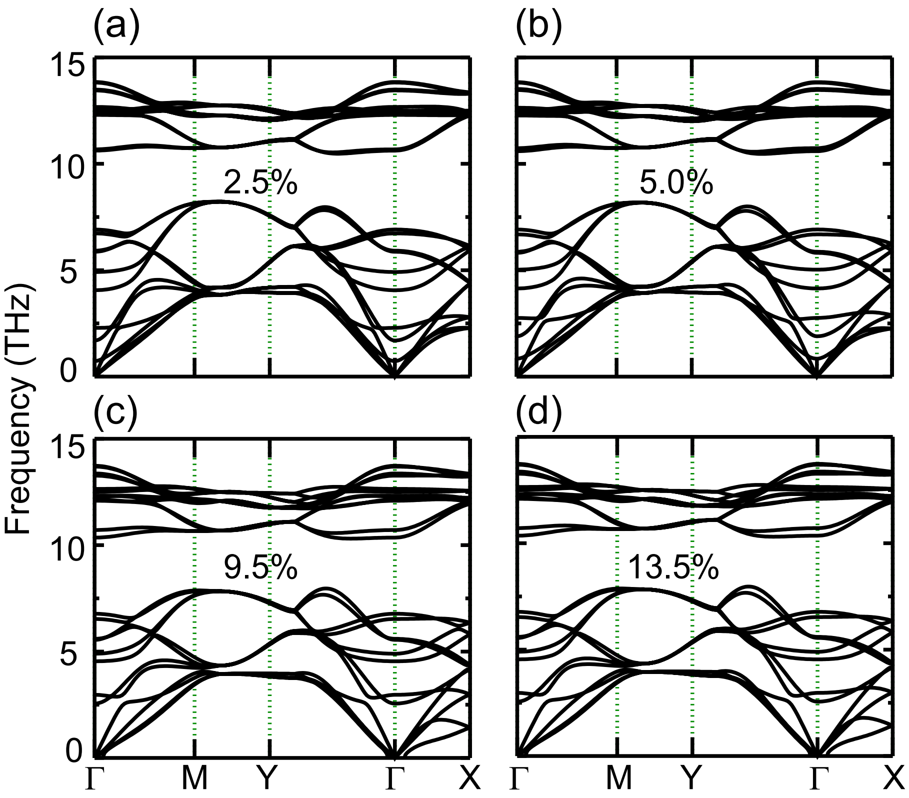


Figure S5: Phonon dispersions for bilayer phosphorene at representative strains, (a) $2.5\%$, (b) $5.0\%$, (c) $9.5\%$, and (d) $13.5\%$. We observe the small imaginary frequency in phonon dispersion at about $15\%$, which is well above the critical strain predicted by PBE as well as HSE06 methods.

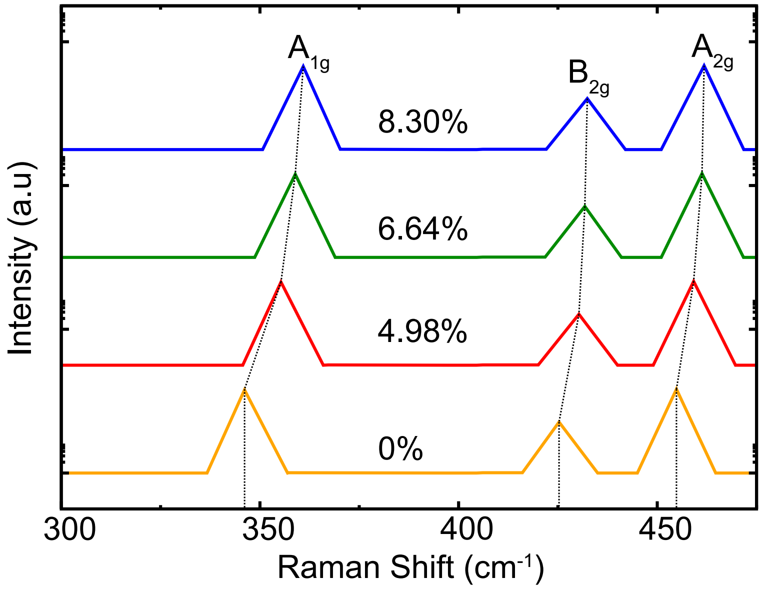


Figure S6: Raman spectra of bilayer phosphorene under NC strain. The peak height is presented in the logarithmic scale. The dashed lines present the change in main three Raman active modes as a function of applied strain. Under NC strain only the out of plane $A_{1g}$ mode changes significantly, whereas, the in-plane modes have a very weak dependence on NC strain.
